# Supplementary material for: MorphStream: Scalable Processing of Transactions over Streams on Multicores
Source: arXiv:2307.12749 source file (2023-07-24)
Supplement: Supplementary file 1 [file appendix.tex]

\begin{comment}
\section{System Architecture}
\label{appendix:architecture}
\system has a novel modularized system architecture with three key components: 
\emph{StreamManager}, 
\emph{TxnManager} and \emph{TxnScheduler}. 
These components are instantiated in each thread locally.
The execution outline of \system is presented in Algorithm~\ref{alg:algo}.
Transactional stream processing is continuous and potentially never ends (Line 1$\sim$8).
The dependency resolution and execution of state transactions are separated into two non-overlapping phases by punctuations~\cite{Tucker:2003:EPS:776752.776780} (Line 2 and 5), which guarantees that no subsequent input event will have a smaller timestamp. 
Effectively, a batch of state transactions is collected during the first phase, and processed during the second phase.

In the first phase (i.e., stream processing phase), 
the \emph{StreamManager} conducts preprocessing for every input event ($e$). Similar to some prior works~\cite{tstream}, state transactions may be issued but not immediately processed during preprocessing (Line 3).
The \emph{pre\_processing} and \emph{post\_processing} functions are exposed as APIs to users.
The \emph{TxnManager} handles dependency resolution (Line 4) among state transactions and insert decomposed operations to construct a \tpg. We discuss the detailed two-phase \tpg construction process in Section~\ref{subsec:construction}.

In the second phase  (i.e., transaction processing phase), 
the \emph{TxnManager} is first involved again to refine (Line 6) the constructed \tpg with further dependency resolution.
The \emph{TxnScheduler} 
schedules operations for concurrent execution based on the constructed \tpg according to the three dimensions of scheduling decisions (Line 7). 
In particular, a scheduling decision model $M$ is instantiated based on the constructed \tpg (Line 14).
\textbf{\circled{1}} Guided by $M$, execution threads adopt an exploration strategy (Section~\ref{subsec:explore}) to explore the constructed \tpg for operations available to be scheduled constrained by dependencies. 
\textbf{\circled{2}} 
During exploration, one or multiple operations may be treated as the 
% basic 
unit of scheduling (Section~\ref{subsec:granularity}). 
Subsequently, \textbf{\circled{3}} every thread executes operation(s) in the unit of scheduling with various abort handling mechanisms (Section~\ref{subsec:abort_handling}).
Only when state transactions are processed (i.e., committed or aborted) can the associated input events be postprocessed (Line 8) by the \emph{StreamManager} based on transaction processing results.
\end{comment}

\begin{comment}
\begin{algorithm}
\footnotesize
    \KwData{$e$ \tcp{Input event}}
    \KwData{$txn_{ts}$ \tcp{State transaction}}
    \KwData{$G$ \tcp{The currently constructed TPG}}
    \While{!finish processing of input streams}{
        \eIf(\tcp*[h]{Phase 1}){\text{$e$ is not a $punctuation$}}{
                $txn_{ts}$ $\gets$ PRE\_Processing($e$)\;
                \textbf{TPG\_Construction}($G$, $txn_{ts}$)\; 
          }(\tcp*[h]{Phase 2}){
                \textbf{TPG\_Refinement}($G$)\; 
                \textbf{TXN\_Scheduling}($G$)\; 
                POST\_Processing()\;
          }
    }
    
    \SetKwFunction{FMain}{TPG\_Construction}
    \SetKwProg{Fn}{Function}{:}{}
    \Fn{\FMain{$G$, $txn_{ts}$}}{
        $O_{1..k}$ $\gets$ \textbf{Partition} $txn_{ts}$\;
        \ForEach{\text{operation $O_{i}$ $\in$ $O_{1..k}$}}{
            \textbf{Identify} its \ld\;
            $G$ $\gets$ $G$ + $O_{i}$ \;
        }
    }
    \SetKwFunction{FMain}{TPG\_Refinement}
    \SetKwProg{Fn}{Function}{:}{}
    \Fn{\FMain{$G$}}{
        \ForEach{\text{vertex $e_{i}$ $\in$ $G$}}{
            \textbf{Identify} its \td, \pd\;
        }
    }
    
    \SetKwFunction{FMain}{TXN\_Scheduling}
    \SetKwProg{Fn}{Function}{:}{}
    \Fn{\FMain{$G$}}{
        $M$ $\gets$ Instantiated with $G$;\tcp{A decision model}
        \While{!finish scheduling of $G$
        }{
          \textbf{\circled{2}} $Scheduling Unit$ $\gets$ \textbf{\circled{1}} \emph{Explore}($G$, $M$)\; 
            \textbf{\circled{3}} \emph{Execute with Abort Handling} ($Scheduling Unit$)\; 
        }
    }
  \caption{Execution Outline of \system}
  \label{alg:algo}
\end{algorithm}
\end{comment}
